# Supplementary material for: Habitat: A Platform for Embodied AI Research
Source: arXiv:1904.01201 source file (2019-11-25)
Supplement: Supplementary file 1 [file supplemental.tex]

\input{preamble}

\iccvfinalcopy

\begin{document}
\input{cover}
\title{\ourtitle\\Supplemental Materials}
\maketitle

\input{supplemental_content}

{\small
\bibliographystyle{ieee_fullname}
\bibliography{biblio}
}

\end{document}
